# Supplementary material for: Liquid interfaces in viscous straining flows: Numerical studies of the selective withdrawal transition
Source: arXiv:physics/0510003 source file (2007-01-21)
Supplement: Supplementary file 1 [file appendix_0.tex]

%auto-ignore
To see why the boundary conditions on $S_R$ are the appropriate
conditions for an effectively infinitely large reservoir, consider the
following  
argument.
